# Supplementary material for: Nonreciprocal interactions drive intermittent melting of Coulomb clusters
Source: arXiv:2602.16074 ancillary file (2026-08-21)
Supplement: Supplementary file 1 [file Supplemental_for_Melting_Coulomb_clusters_through_nonreciprocity_enhanced_parametric_pumping.pdf]

# Supplemental Material for
# Melting Coulomb clusters through nonreciprocity-enhanced parametric pumping

Zhicheng Shu,[1] Wei-Chih Li,[1] Wentao Yu,[2] and Justin C. Burton[1]

[1]*Department of Physics, Emory University*

[2]*Applied Physics and Materials Science, California Institute of Technology*

## CONTENTS

1. Supplemental movies 1

2. Equations of motion in the rotating reference frame 1

3. PCA mode analysis 2

4. Enhanced growth rate due to nonreciprocal interactions 3

## 1. SUPPLEMENTAL MOVIES

Movie S1: 2-particle melted state.
Movie S2: 2-particle quiescent state.
Movie S3: 3-particle melted state.
Movie S4: 3-particle quiescent state.
Movie S5: 7-particle melted state.
Movie S6: 7-particle quiescent state.
Movie S7: 18-particle melted state.
Movie S8: 18-particle quiescent state.
Movie S9: 3-particle quiescent state, in lab frame and the rotating reference frame.
Movie S10: 3-particle melted state, in both experiment and simulation ($\tilde{q} = 0.4, \sigma = 0.1$).

## 2. EQUATIONS OF MOTION IN THE ROTATING REFERENCE FRAME

In this section, we present the equations of motion of a cluster in the rotating reference frame, and show that in the rotating frame the center of mass mode frequency is split due to the Coriolis force, as evident in the mode spectrum in the main text. In the lab inertial reference frame, the horizontal equation of motion is:

$$\ddot{\boldsymbol{\rho}}_i = -\omega_h^2 \boldsymbol{\rho}_i + k_c^2 \hat{z} \times \boldsymbol{\rho}_i + \sum_{j \neq i} f_{ij}^h \hat{\boldsymbol{\rho}}_{ij} - \gamma_i \dot{\boldsymbol{\rho}}_i \tag{S1}$$

where $\boldsymbol{\rho}_i = (x_i, y_i)$, identical to Eq. 1 in the main text, and dotted variables refer to time differentiation. The terms on the right hand side represent: harmonic confinement with fundamental frequency $\omega_h$, non-conservative ion drag force described by $k_c^2$, damping due to neutral gas described by $\gamma_i$, and horizontal pairwise forces between particles $\boldsymbol{f}_{ij}^h = f_{ij}^h \hat{\boldsymbol{\rho}}_{ij}$, which depend on the separation, $\boldsymbol{\rho}_{ij} = \boldsymbol{\rho}_i - \boldsymbol{\rho}_j$.

Next, we want perform a coordinate transformation and write down the equations of motion in a rotating frame with angular velocity $\Omega$. The coordinates transform as $\boldsymbol{\rho} = \mathrm{R}(\Omega t) \cdot \bar{\boldsymbol{\rho}}$, where $\mathrm{R}(\theta) = \begin{bmatrix} \cos\theta & -\sin\theta \\ \sin\theta & \cos\theta \end{bmatrix}$ and $\bar{\boldsymbol{\rho}}$ is the coordinate in the rotating frame. The derivatives of the coordinates transform as: $\frac{d\boldsymbol{\rho}}{dt} = \frac{d}{dt}[\mathrm{R}(\Omega t) \cdot \bar{\boldsymbol{\rho}}] = \Omega \mathrm{R}(\Omega t + \pi/2) \cdot \bar{\boldsymbol{\rho}} + \mathrm{R}(\Omega t) \cdot \frac{d\bar{\boldsymbol{\rho}}}{dt}$, $\frac{d^2\boldsymbol{\rho}}{dt^2} = \frac{d^2}{dt^2}[\mathrm{R}(\Omega t) \cdot \bar{\boldsymbol{\rho}}] = \Omega^2 \mathrm{R}(\Omega t + \pi) \cdot \bar{\boldsymbol{\rho}} + 2\Omega \mathrm{R}(\Omega t + \pi/2) \cdot \frac{d\bar{\boldsymbol{\rho}}}{dt} + \mathrm{R}(\Omega t) \cdot \frac{d^2\bar{\boldsymbol{\rho}}}{dt^2}$. Substituting these into Eq. S1 gives the

equations of motion in terms of coordinates in the rotating frame $\bar{\boldsymbol{\rho}}_i$:

$$\begin{aligned}\frac{d^2\boldsymbol{\rho}}{dt^2} &= \frac{d^2}{dt^2}[\mathrm{R}(\Omega t)\bar{\boldsymbol{\rho}}] = \Omega^2\mathrm{R}(\Omega t+\pi)\bar{\boldsymbol{\rho}} + 2\Omega\mathrm{R}(\Omega t+\pi/2)\frac{d\bar{\boldsymbol{\rho}}}{dt} + \mathrm{R}(\Omega t)\frac{d^2\bar{\boldsymbol{\rho}}}{dt^2} \\ &= -\omega^2\mathrm{R}(\Omega t)\bar{\boldsymbol{\rho}}_i + k_c^2\mathrm{R}(\pi/2)\mathrm{R}(\Omega t)\bar{\boldsymbol{\rho}}_i - \gamma[\Omega\mathrm{R}(\Omega t+\pi/2)\bar{\boldsymbol{\rho}} + \mathrm{R}(\Omega t)\frac{d\bar{\boldsymbol{\rho}}}{dt}] + \sum_j \boldsymbol{f}_{ij}^h.\end{aligned} \tag{S2}$$

By multiplying $\mathrm{R}(-\Omega t)$ on both sides, we end up with the equations of motion in the rotation frame with angular velocity $\Omega$:

$$\Omega^2\mathrm{R}(\pi)\bar{\boldsymbol{\rho}}_i + 2\Omega\mathrm{R}(\pi/2)\frac{d\bar{\boldsymbol{\rho}}_i}{dt} + \frac{d^2\bar{\boldsymbol{\rho}}_i}{dt^2} = -\omega^2\bar{\boldsymbol{\rho}}_i + k_c^2\mathrm{R}(\pi/2)\bar{\boldsymbol{\rho}}_i - \gamma[\Omega\mathrm{R}(\pi/2)]\bar{\boldsymbol{\rho}}_i + \frac{d\bar{\boldsymbol{\rho}}_i}{dt}] + \mathrm{R}(-\Omega t)\sum_j \boldsymbol{f}_{ij}^h \tag{S3}$$

which simplifies to

$$\frac{d^2\bar{\boldsymbol{\rho}}_i}{dt^2} = -(\omega^2-\Omega^2)\bar{\boldsymbol{\rho}}_i - (\gamma\Omega - k_c^2)\hat{z}\times\boldsymbol{\rho}_i - 2\Omega\hat{z}\times\frac{d\bar{\boldsymbol{\rho}}_i}{dt} + \sum_j \bar{\boldsymbol{f}}_{ij}^h \tag{S4}$$

where we have used the relations $\mathrm{R}(\pi)\boldsymbol{\rho} = -\boldsymbol{\rho}, \mathrm{R}(\pi/2)\boldsymbol{\rho} = \hat{z}\times\boldsymbol{\rho}$.

In the main text we have shown that the horizontal center of mass translation modes have split peaks at $\omega_h \pm \Omega$. This can be shown straightforwardly by considering the equation of motion in the rotating reference frame of a particle confined in a harmonic potential:

$$\frac{d^2}{dt^2}\begin{bmatrix} x \\ y \end{bmatrix} = -(\omega_h^2 - \Omega^2)\begin{bmatrix} x \\ y \end{bmatrix} - 2\Omega\frac{d}{dt}\begin{bmatrix} -y \\ x \end{bmatrix}. \tag{S5}$$

By writing $x = Ae^{i(kt+\alpha)}, y = Be^{i(kt+\beta)}$, we get

$$-k^2\frac{d^2}{dt^2}\begin{bmatrix} Ae^{i\alpha} \\ Be^{i\beta} \end{bmatrix} = -(\omega_h^2 - \Omega^2)\begin{bmatrix} Ae^{i\alpha} \\ Be^{i\beta} \end{bmatrix} - 2ik\Omega\begin{bmatrix} -Be^{i\beta} \\ Ae^{i\alpha} \end{bmatrix}. \tag{S6}$$

Defining $\tilde{A} = Ae^{i\alpha}, \tilde{B} = Be^{i\alpha}$, we get

$$\begin{bmatrix} \omega_h^2 - \Omega^2 - k^2 & -2ik\Omega \\ 2ik\Omega & \omega_h^2 - \Omega^2 - k^2 \end{bmatrix}\begin{bmatrix} \tilde{A} \\ \tilde{B} \end{bmatrix} = 0. \tag{S7}$$

Thus the solution for $k$ is determined by $(\omega_h^2 - \Omega^2 - k^2)^2 - 4k^2\Omega^2 = 0$, which gives for solutions of $k$ related to two mode frequencies: $k = \pm(\omega + \Omega)$ and $k = \pm(\omega - \Omega)$.

## 3. PCA MODE ANALYSIS

We use principal component analysis (PCA) as an unbiased method (without estimations on environmental or interaction forces) to derive the oscillation modes, using only the tracked 3D trajectories of the particles. These modes are not necessarily the normal modes of the cluster, rather, they represent oscillation modes that best capture the fluctuations in the positions of the particles relative to their equilibrium configuration. Since the clusters are rotating, we define the equilibrium configuration in the co-rotating reference frame by subtracting the rotation of the clusters. We choose to decompose the oscillation modes into two kinds, horizontal and vertical, since during the stable regime the clusters have well defined 2D structure and their vertical oscillation is mostly decoupled from the horizontal modes.

We start from the tracked 3D trajectories of an $N$-particle cluster over $F$ frames in the rotating frame: $\mathbf{x}(t) = \{x_i(t)\}$, $\mathbf{y}(t) = \{y_i(t)\}$, and $\mathbf{z}(t) = \{z_i(t)\}$, where $i = 1, ..., N$ and $t = 1, ..., F$:

$$D_h[\widetilde{\mathbf{x}}, \widetilde{\mathbf{y}}] = \begin{bmatrix} \widetilde{x}_1(0) & \dots & \widetilde{x}_N(0) & \widetilde{y}_1(0) & \dots & \widetilde{y}_N(0) \\ \vdots & \ddots & \vdots & \vdots & \ddots & \vdots \\ \widetilde{x}_1(F) & \dots & \widetilde{x}_N(F) & \widetilde{y}_1(F) & \dots & \widetilde{y}_N(F) \end{bmatrix}, D_z[\widetilde{\mathbf{z}}] = \begin{bmatrix} \widetilde{z}_1(0) & \dots & \widetilde{z}_N(0) \\ \vdots & \ddots & \vdots \\ \widetilde{z}_1(F) & \dots & \widetilde{z}_N(F) \end{bmatrix}. \tag{S8}$$

TABLE S1. Numerical values of the fitting coefficients. The $n$th order coefficient $f_n$ has the units of $\mathrm{mm}^{-n+1}\cdot\mathrm{s}^{-2}$

| $f_0$ | $f_1$ | $f_2$ | $f_3$ | $f_4$ | $f_5$ | $f_6$ | $f_7$ | $f_8$ | $f_9$ |
|---|---|---|---|---|---|---|---|---|---|
| -26.3 | 254 | $-1.44\times10^3$ | $3.3\times10^3$ | $-3.48\times10^3$ | $6.58\times10^4$ | $-3.99\times10^5$ | $9.39\times10^5$ | $-9.82\times10^5$ | $3.84\times10^5$ |

Here $\widetilde{x}_i(t) = x_i(t) - \bar{x}_i$ represents the fluctuations of the coordinates around their equilibrium (as do $\widetilde{y}_i(t)$ and $\widetilde{z}_i(t)$). We then construct two covariance matrices: one for the horizontal coordinates $\mathbf{x}(t), \mathbf{y}(t)$, and one for the vertical coordinates $\mathbf{z}(t)$:

$$C_h = D_h^T D_h, C_z = D_z^T D_z. \tag{S9}$$

By diagonalizing $C_h$ and $C_z$, we get the eigenvalues $\lambda_k^h$ ($\lambda_k^z$), and eigenvectors $\{\boldsymbol{e}_k^h\}$ ($\{\boldsymbol{e}_k^z\}$) which represent the PCA modes in horizontal (vertical) direction. We can project the trajectories of particles onto the PCA modes and calculate the mode amplitude:

$$S_k^{h,z}(\omega) = \frac{1}{F}\left|\int_0^F e^{i\omega t}\mathbf{P}_k^{h,z}(t)dt\right| \tag{S10}$$

where $\mathbf{P}_k^h(t) = [\widetilde{\mathbf{x}}(t), \widetilde{\mathbf{y}}(t)]\cdot \boldsymbol{e}_k^h$, $\mathbf{P}_k^z(t) = \widetilde{\mathbf{z}}(t)\cdot\boldsymbol{e}_k^z$ are the mode projections in horizontal and vertical direction, respectively. Notice that the variance of the mode projection is equal to the corresponding eigenvalue:

$$\mathrm{Var}(\mathbf{P}_k^{h,z}(t)) = \lambda_k^{h,z}. \tag{S11}$$

Figure. S1 shows the PCA modes of the 7-particle cluster. Fig. S2 shows the mode spectrum. The frequency of the vertical center of mass mode (mode 15) is about twice of that of the breathing mode (mode 2). Figure. S3 shows the PCA modes of the 18-particle cluster. Fig. S4 shows the mode spectrum. The frequency of the vertical center of mass mode (mode 37) is about twice of that of the breathing mode (mode 1). However, notice that the breathing mode here is asymmetric, i.e., the particles in the inner circle and the outer circle oscillate out of phase. Figure S5 shows the PCA modes of the same 18-particle cluster in a slightly different environment (higher pressure and RF power), where the cluster stays in the quiescent state throughout the whole experiment. Figure S6 shows the mode spectrum. There is no signature of parametric coupling between any horizontal and vertical modes.

## 4. ENHANCED GROWTH RATE DUE TO NONRECIPROCAL INTERACTIONS

In this section we examine the instantaneous growth rate prediction from the minimal model. In the main text, we have derived the amplitude-dependent growth rate to be

$$g_{\mathrm{inst}} = -\frac{\gamma}{2} + \sqrt{\left(\frac{a\delta\omega_1}{4\gamma\omega_2}\right)^2 - \frac{\Delta^2}{4} + \frac{\delta\omega_1 f_2|A|^2}{16\omega_2(2g_0+\gamma/2)}}. \tag{S12}$$

In the following, we want to numerically validate the analytical prediction that the nonreciprocal force results in the growth rate increasing quadratically with the mode amplitude. We start by expanding the total interaction force $f_{\mathrm{int}}^z$ measured from simulation. Figure S7 shows the polynomial fit to $f_{\mathrm{int}}^z$ obtained from a simulation with $\tilde{q} = 0.4$ and $\delta = 0.1$. The numerical values of the coefficients of the polynomial are listed in Table S1. For our derivation, we only consider terms up to second order, which describe $f_{\mathrm{int}}^z$ reasonably well for small breathing mode amplitudes ($\approx 0.15$ mm).

For the rest of the parameters appearing in Eq. (S12), we set $\omega_1 = 15\pi$ s$^{-1}$, $\omega_2 = 30\pi$ s$^{-1}$, and $\gamma = 1$ s$^{-1}$. In our 3-particle simulations, the variation of the breathing mode frequency due to the variation of $z_{\mathrm{com}}$ was $\omega_b(z) = \omega_b(0)(1+\alpha z)$, where $\alpha = -0.58$ mm$^{-1}$. Thus $\omega_b^2 \approx \omega_b(0)^2(1+2\alpha z)$, which gives $\delta = 2\alpha = -1.16$ mm$^{-1}$. For the sinusoidal driving strength, $a$, we can write $a = B_0\gamma\omega_2$, where $B_0 = 0.075$ mm represents the steady state oscillation amplitude of $x_2$ when it's only subject to the sinusoidal driving with strength $a$.

We now compare the minimal model prediction of the breathing mode growth to simulations. In Fig. S9, we show the evolution of the cluster radius $R$, and the vertical center of mass $z_{\mathrm{com}}$, in a simulation with nonreciprocal interactions. At $t \approx 4$ s, the breathing mode starts to grow. By fitting the slope of the breathing mode amplitude (defined as the half peak to peak oscillation amplitude of $R$) over time on a log linear scale, we notice two regimes. From $t \approx 4$ s to $t \approx 7.5$ s, the breathing mode grows with growth rate $\approx 0.56$ s$^{-1}$. From $t \approx 7.5$ s to $t \approx 10$ s,

the breathing mode grows with growth rate $\approx 0.99$ s$^{-1}$. The enhancement of the growth rate between $t \approx 7.5$ s and $t \approx 10$ is also accompanied by the increase of vertical oscillation amplitude. In Fig. S9(b), the cyan dashed line represent amplitude of 0.036 mm, which is the minimal amplitude required to have a positive $g_0$ (Fig. S8), while the black dashed line represent the amplitude of 0.075 mm, which gives $g_0 = 0.52$ s$^{-1}$. This suggests that the dynamics observed in the simulation with nonreciprocal interactions agrees with our model prediction. Before $t \approx 4$ s, the vertical oscillation amplitude is consistently below the threshold for positive $g_0$, thus the breathing mode does not grow. At $t \approx 4$ s, the vertical oscillation amplitude surpasses the threshold for positive $g_0$ and remains so for a few seconds, thus the breathing mode grows and the growth rate is consistent with $g_0$ at this $z$ amplitude. As the breathing mode amplitude continues to increase, the breathing mode growth rate transitions to $\approx 1$ s$^{-1}$, which is close to the value of $g_{\rm inst}$ with $|A| \approx 0.2$ mm. Unlike the minimal model where $x_1$ and $x_2$ blow up, in simulations the growth of the breathing mode faces nonlinearity at large amplitude and is eventually terminated by the cluster melting, as indicated by the switching of $w_3$.

In comparison, in Fig. S10, we show the same analysis for a simulation with reciprocal interactions, but with significantly larger noise strength. In this case, we notice that the vertical oscillation amplitude has larger variations due to larger noise. This results in larger variations of $R$ around its equilibrium, and the measured growth rate matches the predicted value of $g_0$ at vertical oscillation amplitude $\approx 0.15$ mm.

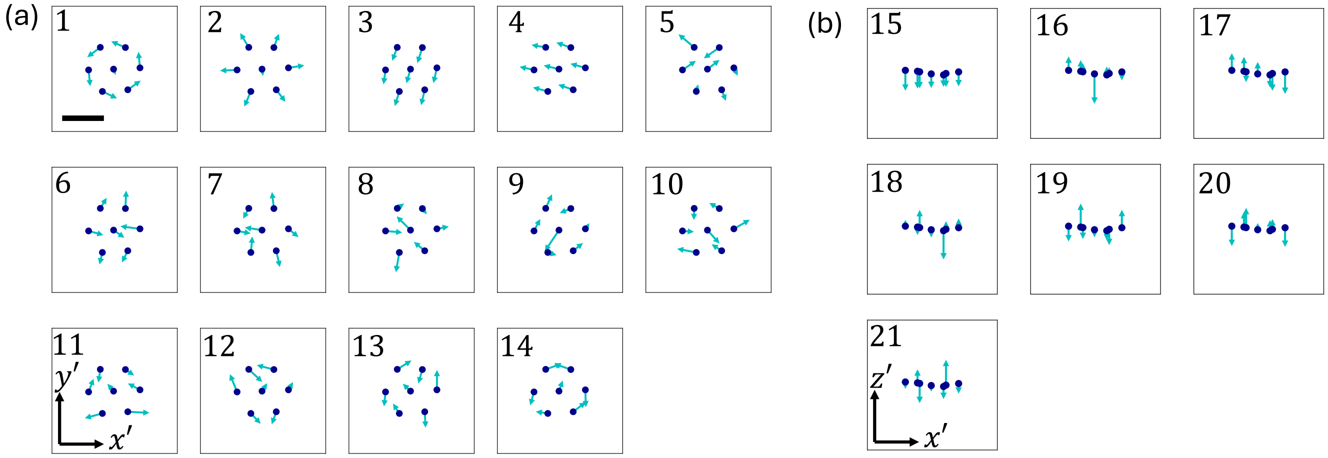


FIG. S1. PCA modes of the 7-particle cluster.

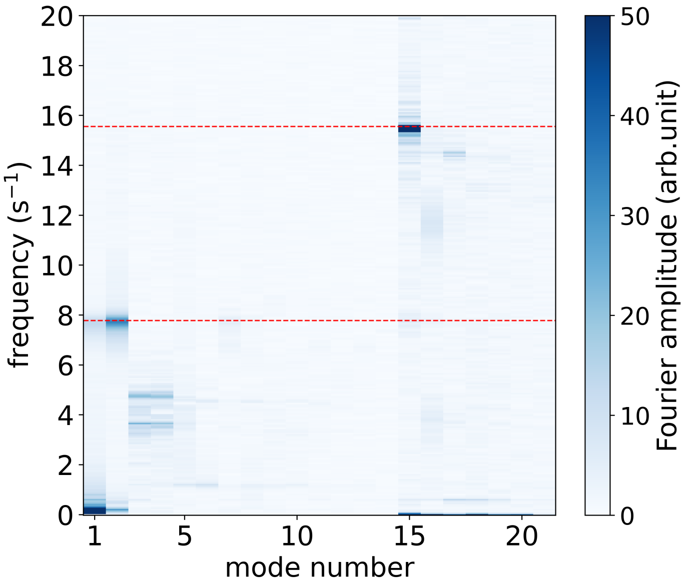


FIG. S2. Mode spectrum of the 7-particle cluster. The two red dashed lines represent the frequency of the vertical center of mass mode frequency (mode 15) and half of that frequency.

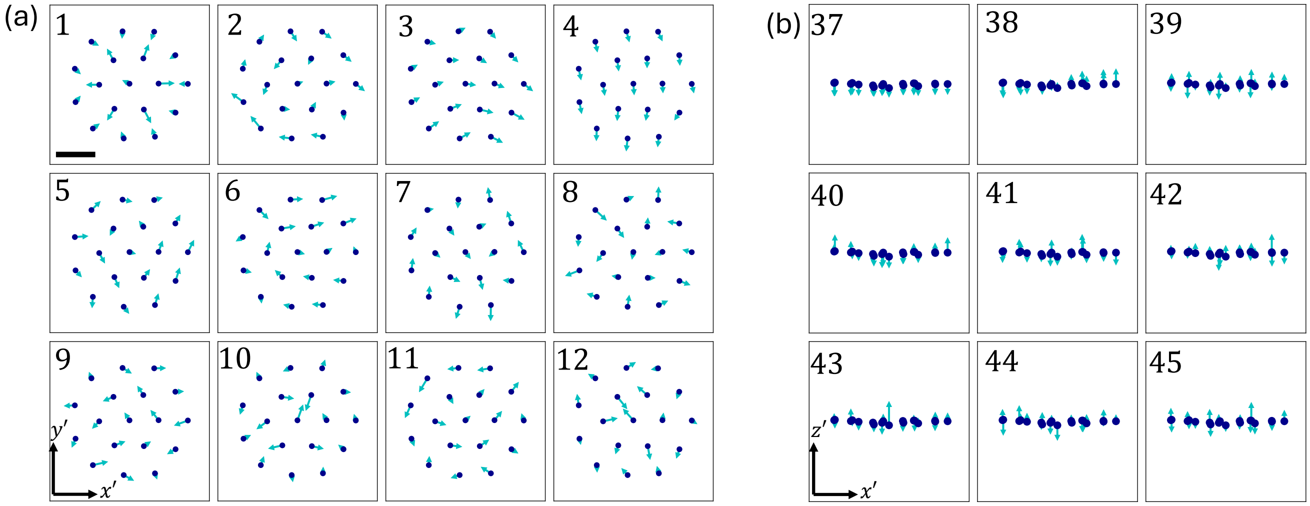


FIG. S3. PCA modes of the 18-particle cluster.

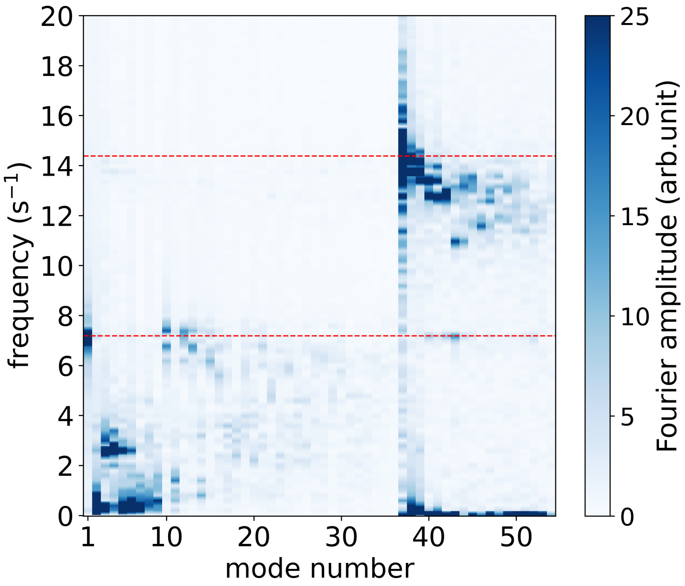


FIG. S4. Mode spectrum of the 18-particle cluster. The two red dashed lines represent the frequency of the vertical center of mass mode frequency (mode 37) and half of that frequency.

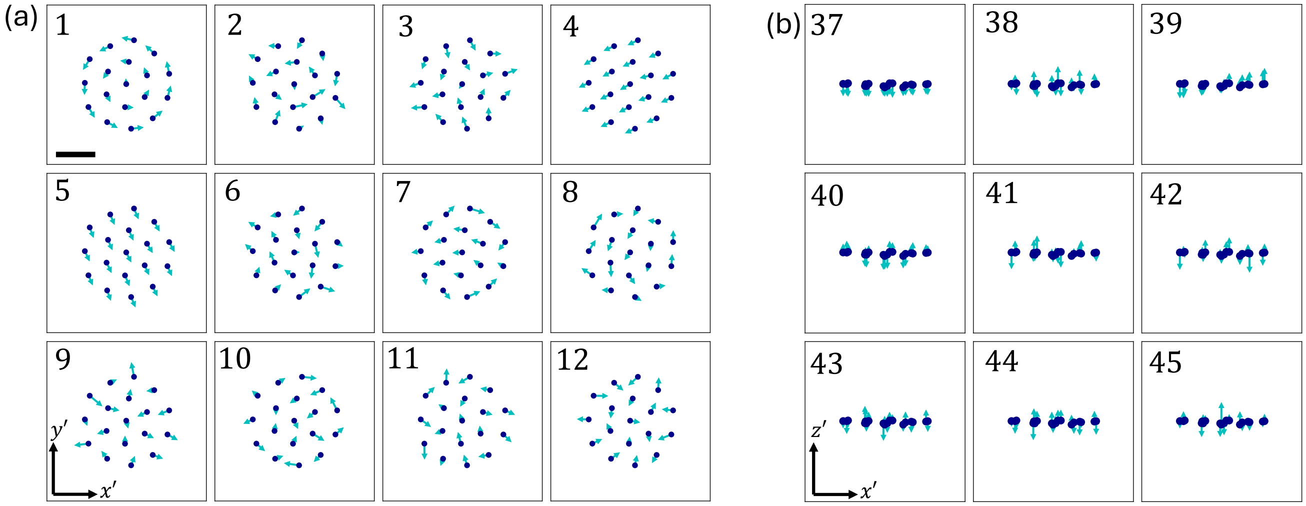


FIG. S5. PCA modes of the 18-particle cluster.

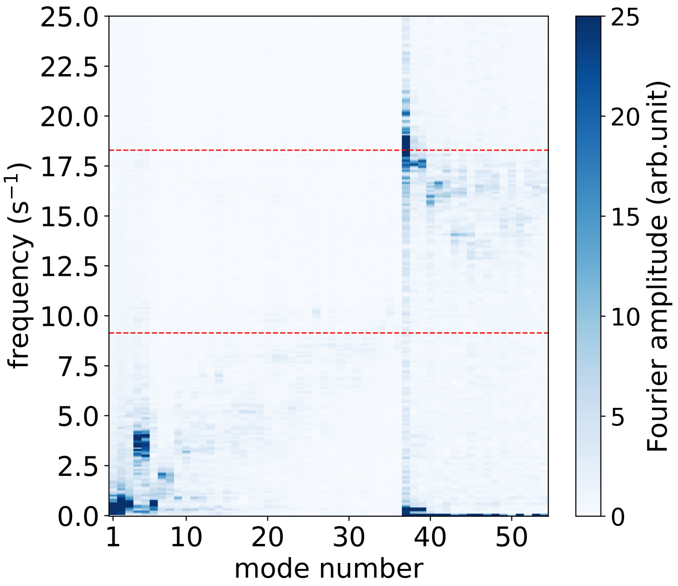


FIG. S6. Mode spectrum of the 18-particle cluster that doesn't display intermittent melting. The two red dashed lines represent the frequency of the vertical center of mass mode frequency (mode 37) and half of that frequency.

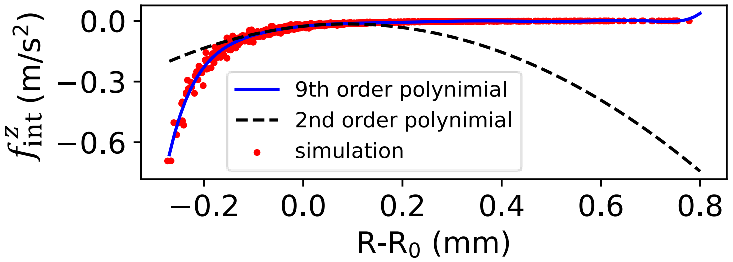


FIG. S7. Polynomial fits to the total $z$ interaction force in the simulation with $\tilde{q} = 0.4$ and $\delta = 0.1$. The data is also shown in Fig. 6c in the main text.

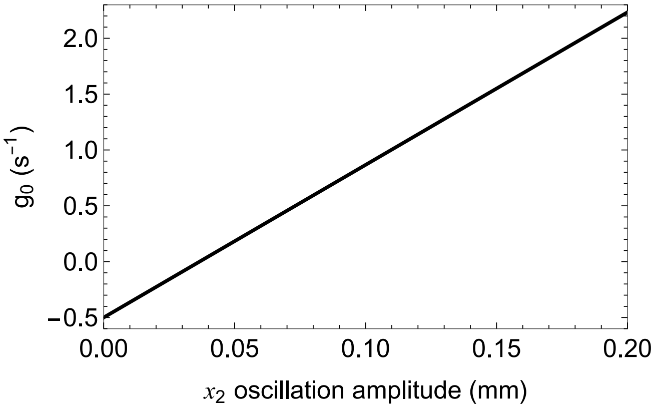


FIG. S8. Growth rate $g_0$ versus the oscillation amplitude of $x_2$ in the absence of nonreciprocity, $f(x_1)$.

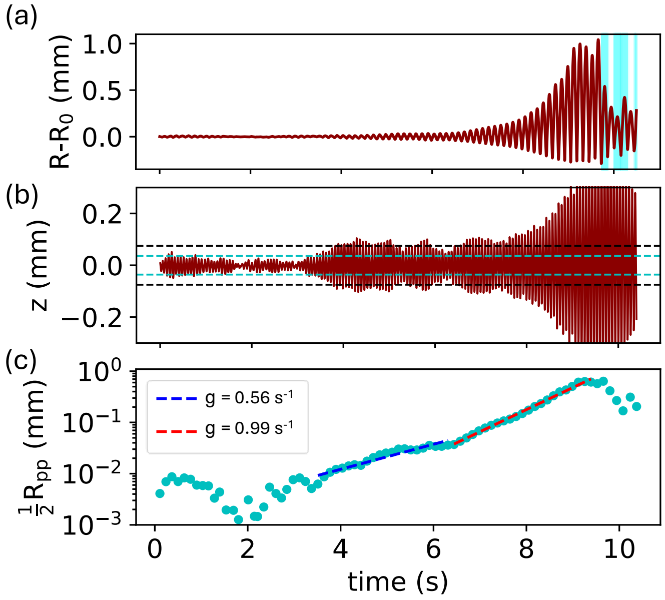


FIG. S9. Growth of breathing mode amplitude in simulation with $\tilde{q} = 0.4$, $\sigma = 0.1$. (a) Change of cluster radius $R$ from its equilibrium value $R_0$. The blue shaded regions indicate $w_3 < 0$. (b) Vertical center of mass position of the cluster. The cyan and black dashed lines indicate oscillation amplitudes of 0.036 mm and 0.075 mm, respectively. (c) Breathing mode amplitude versus time plotted in log-linear scale. The blue and red dashed lines represent linear fits that produce growth rates of 0.56 s$^{-1}$ and 0.99 s$^{-1}$, respectively.

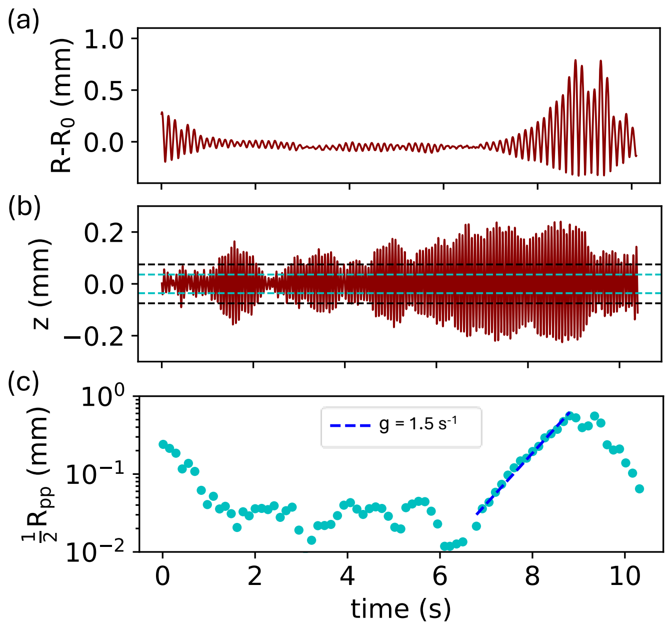


FIG. S10. Growth of breathing mode amplitude in simulation with $\tilde{q} = 0$, $\sigma = 0.25$. (a) Change of cluster radius $R$ from its equilibrium value $R_0$. (b) Vertical center of mass position of the cluster. The cyan and black dashed lines indicate oscillation amplitudes of 0.036 mm and 0.147 mm, respectively. (c) Breathing mode amplitude versus time plotted in log-linear scale. The blue line represents linear fit that produces growth rate of 1.5 $s^{-1}$.
